# Supplementary material for: ORCNet: A context-based network to simultaneously segment the ocular region components
Source: arXiv:2204.07456 source file (2022-04-15)
Supplement: Supplementary file 1 [file text.tex]

%!TEX root = ../../main.tex

\appendices
\section{Proof of the First Zonklar Equation}
Appendix one text goes here.

% you can choose not to have a title for an appendix
% if you want by leaving the argument blank
\section{}
Appendix two text goes here.
